# Supplementary material for: RPM: Generalizable Behaviors for Multi-Agent Reinforcement Learning
Source: arXiv:2210.09646 source file (2022-10-18)
Supplement: Supplementary file 1 [file appendix.tex]

\newpage
\appendix
